# Supplementary material for: Suppression of the skyrmion Hall effect in planar nanomagnets by the magnetic properties engineering: Skyrmion transport on nanotracks with magnetic strips
Source: arXiv:1912.03403 source file (2020-02-14)
Supplement: Supplementary file 1 [file Supplementary_Material.pdf]

# Supplementary Material

## Suppression of the skyrmion Hall effect in planar nanomagnets by the magnetic properties engineering: Skyrmion transport on nanotracks with magnetic strips

D. Toscano,[1, a)] J.P.A. Mendonça,[1] A.L.S. Miranda,[1] F. Sato,[1] P. Z. Coura,[1] and S. A. Leonel[1]

*Departamento de Física, Laboratório de Simulação Computacional, Universidade Federal de Juiz de Fora, Juiz de Fora, Minas Gerais 36036-330, Brazil*

(Dated: January 20, 2020)

Micromagnetic simulations have been performed to investigate the suppression of the skyrmion Hall effect in nanotracks with their magnetic properties strategically modified. In particular, we study two categories of magnetically modified nanotracks. One of them, repulsive edges have been inserted in the nanotrack and, in the other, an attractive strip has been placed exactly on the longest axis of the nanotrack. Attractive and repulsive interactions can be generated from the engineering of magnetic properties. For instance, it is known that the skyrmion can be attracted to a region where the exchange stiffness constant is decreased. On the other hand, the skyrmion can be repelled from a region characterized by a local increase in the exchange stiffness constant. In order to provide a background for experimental studies, we vary not only the magnetic material parameters (exchange stiffness, perpendicular magnetocrystalline anisotropy and the Dzyaloshinskii-Moriya constant) but also the width of the region magnetically modified, containing either a local reduction or a local increase for each one of these magnetic properties. In the numerical simulations, the skyrmion motion was induced by a spin-polarized current and the found results indicate that it is possible to transport skyrmions around the longest axis of the nanotrack. In practice, the skyrmion Hall effect can be completely suppressed in magnetic nanotracks with strategically modified magnetic properties. Furthermore, we discuss in detail 6 ways to suppress the skyrmion Hall effect by the usage of nanotracks with repulsive edges and nanotracks with an attractive strip.

[a)] Electronic mail: dtoscano@ice.ufjf.br

Several works have ignored the dipolar interaction when dealing with magnetic thin films with high PMA and interfacial Dzyaloshinskii-Moriya interactions, whereas others argue that the effect of the dipolar coupling can be incorporated in the effective anisotropy.

In this supplementary material we describe carefully the Methodology used in manuscript, besides providing additional simulations that include or not the effect of the full dipolar coupling. When comparing these simulations, we provide our justification for including the effect of the shape anisotropy into an effective anisotropy.

To describe the magnetic system we have considered exchange, Dzyaloshinskii-Moriya, perpendicular magnetic anisotropy (PMA) and dipole-dipole interactions, included in the following Hamiltonian:

$$\begin{aligned} \mathscr{H} = & -\mathcal{C}^{\text{EXC}} \sum_{<i,j>} [\, \hat{m}_i \cdot \hat{m}_j \,] \; + \\ & -\mathcal{C}^{\text{DMI}} \sum_{<i,j>} \left[ \hat{d}_{ij} \cdot (\hat{m}_i \times \hat{m}_j) \right] \; + \\ & -\mathcal{C}^{\text{PMA}} \sum_{i} [\, \hat{m}_i \cdot \hat{n} \,]^2 \; + \\ & -\mathcal{C}^{\text{DIP}} \sum_{i,j} \left[ \frac{3(\hat{m}_i \cdot \hat{r}_{ij})(\hat{m}_j \cdot \hat{r}_{ij}) - \hat{m}_i \cdot \hat{m}_j}{(r_{ij}/a)^3} \right] \end{aligned} \tag{S1}$$

where $\hat{m}_i = (m_i^x, m_i^y, m_i^z)$ is the unit vector which represents the magnetic moment located at the $i$ site located by position vector $\vec{r}_i = (x_i, y_i, z_i)$. The versor $\hat{r}_{ij} = \dfrac{\vec{r}_i - \vec{r}_j}{|\vec{r}_i - \vec{r}_j|}$ is directed along the direction which join the sites $i$ and $j$, being $r_{ij} = |\vec{r}_i - \vec{r}_j|$ the relative distance between them. $a$ represents lattice parameter. The strength of the magnetic interactions have the same dimension, that is, $\mathcal{C}^{\text{EXC}}$, $\mathcal{C}^{\text{DMI}}$, $\mathcal{C}^{\text{PMA}}$ and $\mathcal{C}^{\text{DIP}}$ in units of energy (J). In the micromagnetic approach, the renormalization of magnetic interaction constants depend not only on the parameters of the material, but also on the manner in which the system is partitioned into cells. As in many micromagnetic simulation packages, we have used in our simulations the finite difference method, which subdivides the simulated geometry into cubic cells, that is, $V_{\text{cel}} = a^3$. In this case, magnetic interaction constants are as follow:

$$\mathcal{C}^{\text{EXC}} \;=\; J \;= 2\, a\, A \tag{S2}$$

$$\mathcal{C}^{\,\mathrm{DMI}} \;=\; a^2\,D \tag{S3}$$

$$\mathcal{C}^{\,\mathrm{PMA}} \;=\; a^3\,K_{\mathrm{u}} \tag{S4}$$

$$\mathcal{C}^{\,\mathrm{DIP}} \;=\; \frac{\mu_0\,a^3}{4\pi}\,M_{\mathrm{S}}^2 \tag{S5}$$

where $A$, $D$, $K_{\mathrm{u}}$ and $M_{\mathrm{S}}$ are material parameters: exchange stiffness constant, Dzyaloshinskii-Moriya constant, magnetocrystalline anisotropy and saturation magnetization, respectively. Each micromagnetic cell hosts an effective magnetic moment $\vec{m}_i = (M_{\mathrm{S}} V_{\mathrm{cel}})\hat{m}_i$ aligned to the direction in which the atomic moments are saturated. It is convenient to use reduced units, from which the definition of the characteristic lengths emerges. To compute the system energy we use units of the cell-to-cell exchange constant $\mathcal{C}^{\,\mathrm{EXC}} \;=\; J \;= 2\,a\,A$. Thus, we can write

$$\frac{\mathcal{C}^{\,\mathrm{DMI}}}{\mathcal{C}^{\,\mathrm{EXC}}} \;=\left(\frac{a}{\xi}\right) \tag{S6}$$

$$\frac{\mathcal{C}^{\,\mathrm{PMA}}}{\mathcal{C}^{\,\mathrm{EXC}}} \;=\; \frac{1}{2}\left(\frac{a}{\Delta}\right)^2 \tag{S7}$$

$$\frac{\mathcal{C}^{\,\mathrm{DIP}}}{\mathcal{C}^{\,\mathrm{EXC}}} \;=\; \frac{1}{4\pi}\left(\frac{a}{\lambda}\right)^2 \tag{S8}$$

where $\lambda = \sqrt{\dfrac{2A}{\mu_0 M_{\mathrm{S}}^2}}$ is the exchange length, $\Delta = \sqrt{\dfrac{A}{K_{\mathrm{u}}}}$ is the wall width parameter and $\xi = \frac{2A}{D}$ is the characteristic length associated with the Dzyaloshinskii-Moriya interaction. Typical parameters for Co/Pt multilayers have been used in our simulations, the values are as follow: exchange stiffness constant $A = 1.5 \times 10^{-11}$ J/m, Dzyaloshinskii-Moriya constant $D = 3.0 \times 10^{-3}$ J/m$^2$, magnetocrystalline anisotropy constant $K_{\mathrm{u}} = 8.0 \times 10^5$ J/m$^3$ and saturation magnetization $M_{\mathrm{S}} = 5.8 \times 10^5$ A/m. In order to choose a suitable size for the work cell we estimate the characteristic lengths that are relevant to the problem: $\lambda \approx 8.42$ nm, $\Delta \approx 4.33$ nm and $\xi \approx 10.0$ nm. Based on these estimates, the size of the work cell used in the simulations was $V_{\mathrm{cel}} = (2 \times 2 \times 2)$ nm$^3$. Once the side of the cell is smaller than the smallest characteristic lengths, $a = 2$ nm $< \Delta$, the chosen micromagnetic cell is accurate enough for the current study. For the geometric parameters of the planar nanowires we have considered the length $L_x = 1000$ nm, the width $L_y = 100$ nm and the thickness $L_z = 2$ nm.

Once $\mathcal{C}^{\text{EXC}} > 0$, the first term in Eq. (S1) describes the ferromagnetic coupling (isotropic Heisenberg model). Due to the short range of the exchange interaction, the summation is over the nearest magnetic moment pairs $< i, j >$. For the work cell size and material parameters above-mentioned we have estimated $\frac{\mathcal{C}^{\text{DMI}}}{\mathcal{C}^{\text{EXC}}} = 2.00 \times 10^{-1}$, $\frac{\mathcal{C}^{\text{PMA}}}{\mathcal{C}^{\text{EXC}}} \approx 1.07 \times 10^{-1}$ and $\frac{\mathcal{C}^{\text{DIP}}}{\mathcal{C}^{\text{EXC}}} \approx 4.48 \times 10^{-3}$. This makes evident the strength of magnetic interactions in relation to exchange interaction; the strongest interaction. In order of decreasing magnitude: $\mathcal{C}^{\text{EXC}} > \mathcal{C}^{\text{DMI}} > \mathcal{C}^{\text{PMA}} > \mathcal{C}^{\text{DIP}}$. In the second term of Eq. (S1), the versor $\hat{d}_{ij}$ depends on the type of the Dzyaloshinskii-Moriya interaction that the system presents, which can be either intrinsic in chiral magnets or induced in magnetic multilayer systems with broken inversion symmetry and strong spin-orbit coupling. For this reason, there are two types of skyrmions: Bloch skyrmions (vortex-type configuration) and Néel skyrmions (hedgehog-type configuration). Usually Bloch skyrmions arise in magnetically ordered systems with intrinsic Dzyaloshinskii-Moriya interaction (bulk materials), whereas the nucleation of Néel skyrmions is favored by the interfacially induced Dzyaloshinskii-Moriya interaction (magnetic multilayer with high perpendicular magnetocrystalline anisotropy). In summary, the versor of the Dzyaloshinskii-Moriya interaction determines the quasiparticle topology:

$$\hat{d}_{ij} = \begin{cases} \hat{u}_{ij} & \text{Bloch skyrmions - rotational symmetry} \\ \hat{u}_{ij} \times \hat{z} & \text{Néel skyrmions - radial symmetry} \end{cases} \tag{S9}$$

where $\hat{u}_{ij}$ is unit vector joining the sites $i$ and $j$ in the same layer. The third term in Eq. (S1) describes the uniaxial magnetocrystalline anisotropy, since $\mathcal{C}^{\text{PMA}} > 0$ and $\hat{n} = \hat{z}$ being a versor perpendicular to the magnetic layer surface. The last term in Eq. (S1) represents the dipolar coupling. The parameter of the dipolar interaction is always positive ($\mathcal{C}^{\text{DIP}} > 0$), thus one can see that its last term tends to align the magnetic moments anti-ferromagnetically, whereas the first one tends to align the magnetic moments along the direction which couple them $\hat{r}_{ij}$. The dipole-dipole interactions are responsible by the origin of the shape anisotropy. In soft ferromagnetic magnetic, like Permalloy, the magnetocrystalline anisotropy is negligible. Thus, the shape anisotropy dominates the effective anisotropy and the dipolar coupling should be carefully considered in order to describe accurately a nanoscaled soft magnet. Due to the long-range of the dipole-dipole interactions, the magnetostatic coupling cannot be underestimated. For example, the remanent state of an elongated soft nanomagnet can be a single-domain (quasi-uniform state). In this case, the shape anisotropy imposes a magneti-

zation easy axis, being the term $\left[\frac{3(\hat{m}_i\cdot\hat{r}_{ij})(\hat{m}_j\cdot\hat{r}_{ij})}{(r_{ij}/a)^3}\right]$ responsible by the origin of the alignment of the magnetic moments along the longest axis of the nanomagnet. On the other hand, in ultra-thin films with high magnetocrystalline anisotropy (like Co/Pt multilayers used in our simulations), the magnetization easy axis is perpendicular to the magnetic layer surface. As we have previously estimated, the magnetocrystalline anisotropy constant $\mathcal{C}^{\,\text{PMA}}$ is one order of magnitude larger than the dipolar coupling constant $\mathcal{C}^{\,\text{DIP}}$. Thus, the magnetocrystalline anisotropy dominates the effective anisotropy. Besides being responsible by the alignment along the longest axis of the nanomagnet, it is very well-known the effect induced by the dipolar coupling in ultra-thin films favors the confinement the magnetic moments inside the plane of the nanomagnet. In other words, the dipolar coupling can work as an easy-plane anisotropy. It can be written as a Hamiltonian model

$$\mathscr{H}^{\,\text{anis}}_{\,\text{shape}} \;=\; + \left(\frac{\mu_0\, M_{\text{S}}^2}{2}\right) a^3 \sum_i \,[\,\hat{m}_i\cdot\hat{n}\,]^2 \tag{S10}$$

where $\hat{n}=\hat{z}$ gives the direction of the magnetization hard axis.

Although we have not taken into account the full dipolar coupling in the simulations of the manuscript, we took into account the shape anisotropy of a planar nanomagnet by considering an effective uniaxial anisotropy[1], that is

$$K = K_{\text{u}} - \frac{\mu_0\, M_{\text{S}}^2}{2} \tag{S11}$$

More specifically, we have considered the following a Hamiltonian model, which describes an effective uniaxial anisotropy

$$\mathscr{H}^{\,\text{anis}}_{\,\text{eff}} \;=\; -K_{\text{u}}\, a^3 \sum_i \,[\,\hat{m}_i\cdot\hat{n}\,]^2 \;+ \left(\frac{\mu_0\, M_{\text{S}}^2}{2}\right) a^3 \sum_i \,[\,\hat{m}_i\cdot\hat{n}\,]^2$$

That is,

$$\mathscr{H}^{\,\text{anis}}_{\,\text{eff}} \;=\; -\,a^3\left[K_{\text{u}} \;-\; \frac{\mu_0\, M_{\text{S}}^2}{2}\right]\sum_i \,[\,\hat{m}_i\cdot\hat{n}\,]^2 \;=\; -\,a^3\,K\sum_i \,[\,\hat{m}_i\cdot\hat{n}\,]^2 \tag{S12}$$

If, on the one hand, the full dipolar coupling is accurate enough to describe the shape anisotropy in nanomagnets. On the other hand, much time is taken to compute all the dipole-dipole interactions. As previously estimated, the strength of the dipolar coupling is the weakest, about 3 orders of magnitude smaller than the exchange coupling, that is, $\frac{\mathcal{C}^{\,\text{DIP}}}{\mathcal{C}^{\,\text{EXC}}} \approx 4.48\times 10^{-3}$.

In the light of these considerations, we investigate the effect of the dipolar coupling in magnetic thin films with high PMA and interfacial Dzyaloshinskii-Moriya interactions, when comparing simulations in the presence and absence of the dipole-dipole interactions. As we have already discussed the methodology to solve the LLG equation in the manuscript, Here, we restrict to present the results of micromagnetic simulations not only for relaxation simulations, but also those involving the skyrmion transport in nanotracks.

Fig.(S1) shows the out-of-plane magnetization profiles, including or not the full dipolar coupling. As a first approximation, the shape anisotropy has been considered in the effective anisotropy $K = K_u - \frac{\mu_0 M_S^2}{2}$, such as suggested in Ref.[1]. For Co/Pt ultrathin films, we compute $K = 5.9 \times 10^5$ J/m$^3$. Unless otherwise stated, this value for the effective uniaxial anisotropy constant was used in most of our simulations. From this figure, one can see that the profiles of the skyrmions are very similar.

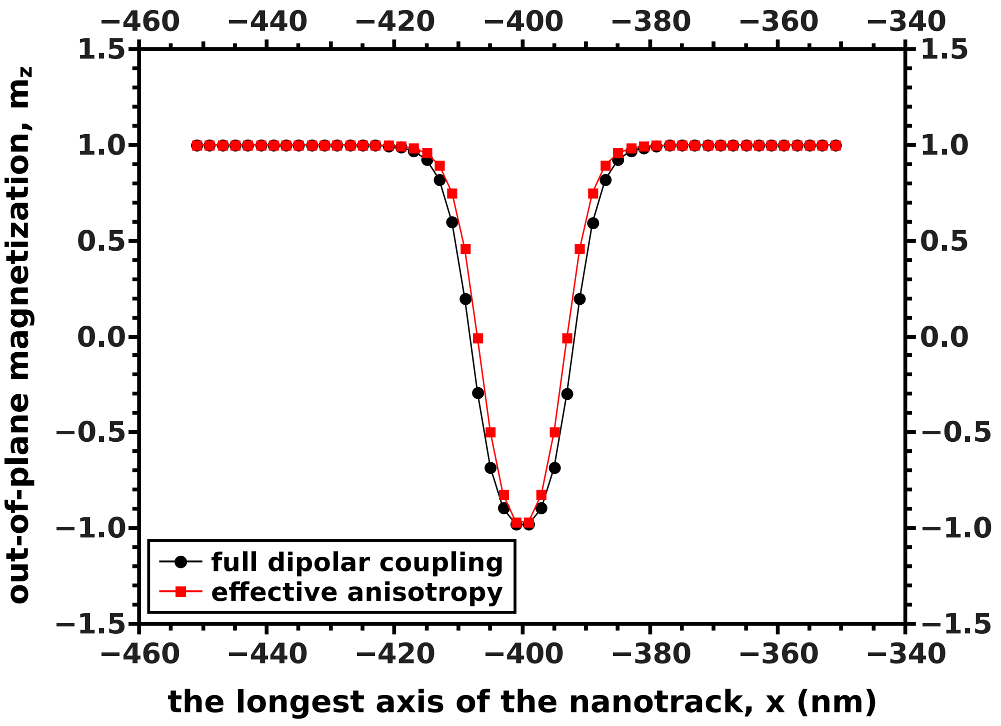


Figure S1. Micromagnetic simulations of relaxation. After the the relaxation process to be finished, we plot the skyrmion profile. In these simulations, we obtain a skyrmion at the position $(X_S, Y_S) = (-400, 0)$ nm, as discussed in the manuscript.

Next, we apply a spin-polarized current in order to move the skyrmion from the left to the right. The skyrmion trajectories are shown in Fig. (S2). One can see that the effective anisotropy modifies slightly the skyrmion trajectory.

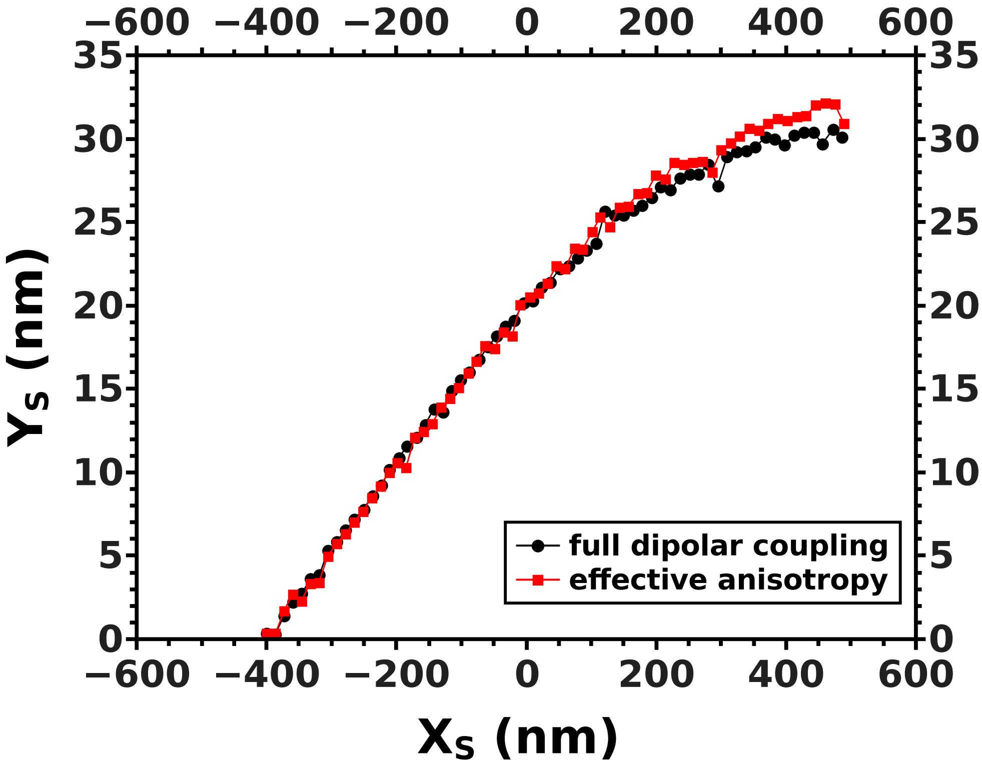


Figure S2. Micromagnetic simulations of the dynamics of the skyrmion driven by a spin-polarized current. Here, we can observe the skyrmion Hall effect.

Therefore, we show that including or not the effect of the full dipolar coupling, the results of the micromagnetic simulations remain qualitatively the same for simulated nanotrack, provided the shape anisotropy be included in the effective anisotropy and the skyrmion trajectory be distant from the boundary of the sample.

It is worth mentioning that the incorporation of the dipolar coupling in the effective uniaxial anisotropy is a usual practice[1–4], which has been used in the majority of micromagnetic simulations similar to ours. Sampaio et al.[4] highlight that dipolar interactions were taken into account, but they found them to have negligible influence. Furthermore, this observation has been reported by other independent teams[1,5,6].

As above-discussed as well as in in the manuscript, the dipolar coupling in ultra-thin films favors the confinement the magnetic moments inside the plane of the nanomagnet. In other words, the dipolar coupling works as an easy-plane anisotropy. Essentially, the confinement of the skyrmion in the nanomagnets is not linked to the dipolar coupling. As reported in a number of papers, see for example Refs.[1,3], the Dzyaloshinskii-Moriya interaction is fundamental to describe the effect of the sample edge on the confinement of the skyrmion. Furthermore, the Ref.[7] highlights that the edge potential it is not of dipolar coupling origin. However, Figure (S2) shows that dipolar coupling is also responsible in part for the skyrmion-edge interaction. As we have point out, the skyrmion-edge interaction is still controversial. In a future work, we intend to investigate this subject carefully.

Nowadays, several micromagnetic softwares (available in free as well as commercial versions) have been used to solve the Landau-Lifshitz-Gilbert equation. Naturally, before the appearance of specialized simulation codes, theoretical researchers in Magnetism had to developed their own micromagnetic codes and it was not a problem to advance in the research. Quite the opposite, a tool to predict experimental observations. The micromagnetic simulation packages, such as OOMMF, MuMax, Magpar and NMag are widely accepted in the scientific community, because they have reproduced several experimental results. As an alternative to the above-mentioned specialized simulation codes, we have been developing a computational code to solve the Landau-Lifshitz-Gilbert equation. Although many of these specialized simulation codes are open-source, we feel more comfortable to include implementations (such as magnetic or geometric defects in the simulated nanomagnet) in our computational code. Thus, we know exactly what we are doing, once we have total control over the code. The validity of results obtained through numerical simulations must always be questioned. During the last few years, we have tested our micromagnetic code in several nanoscaled magnetic systems, such as nanodisks, nano-ellipses and nanowires, and the magnetization dynamics of a single-domain[8,9], vortices[10,11], skyrmions[12] and domain walls[13–15] has been reproduced, being in agreement with experimental observations as well as the predictions of other micromagnetic softwares. Thus, we can state that the computational code is calibrated to reproduce and predict the magnetization dynamics in nanomagnets.

## REFERENCES


[1]S. Rohart, A. Thiaville, Skyrmion confinement in ultrathin film nanostructures in the presence of Dzyaloshinskii-Moriya interaction, Phys. Rev. B 88 (2013) 184422.

[2]S. Heinze, K. von Bergmann, M. Menzel, J. Brede, A. Kubetzka, R. Wiesendanger, G. Bihlmayer, S. Blüge, Spontaneous atomic-scale magnetic skyrmion lattice in two dimensions, Nature Phys. 7 (2011) 713-718.

[3]J. Iwasaki, M. Mochizuki, N. Nagaosa, Current-induced skyrmion dynamics in constricted geometries, Nat. Nanotechnol. 8 (2013) 742-747.

[4]J. Sampaio, V. Cros, S. Rohart, A. Thiaville, A. Fert, Nucleation, stability and current-induced motion of isolated magnetic skyrmions in nanostructures, Nat. Nanotechnol. 8 (2013) 839-844.

[5]Y. Zhou, M. Ezawa, A reversible conversion between a skyrmion and a domain-wall pair in a junction geometry, Nat. Commun. 5 (2014) 4652.

[6]Y.M. Luo, C. Zhou, C. Won, Y.Z. Wu, Magnetic vortex gyration affected by Dzyaloshinskii-Moriya interaction, J. Appl. Phys. 117 (2015) 163916.

[7]J.C. Martinez, W.S. Lew, W.L. Gan, M.B.A. Jalil, Theory of current-induced skyrmion dynamics close to a boundary, J. Magn. Magn. Mater. 465 (2018) 685-691.

[8]D.S. Vieira Júnior, S.A. Leonel, R.A. Dias, D. Toscano, P.Z. Coura, F. Sato, Ground state study of the thin ferromagnetic nano-islands for artificial spin ice arrays, J. Appl. Phys. 116 (2014) 093901.

[9]D.S. Vieira Júnior, S.A. Leonel, D. Toscano, F. Sato, P.Z. Coura, R.A. Dias, Study on the coherence degree of magnetization reversal in Permalloy single-domain nano-ellipses, J. Magn. Magn. Mater. 426 (2017) 396-404.

[10]D. Toscano, S.A. Leonel, P.Z. Coura, F. Sato, R.A. Dias, B.V. Costa, Dynamics of the vortex core in magnetic nanodisks with a ring of magnetic impurities, Appl. Phys. Lett. 101 (2012) 252402.

[11]J.H. Silva, D. Toscano, F. Sato, P.Z. Coura, B.V. Costa, S.A. Leonel, The influence of magnetic impurities in the vortex core dynamics in magnetic nano-disks, J. Magn. Magn. Mater. 324 (2012) 3083-3086.

[12]D. Toscano, S.A. Leonel, P.Z. Coura, F. Sato, Building traps for skyrmions by the incorporation of magnetic defects into nanomagnets: Pinning and scattering traps by magnetic

properties engineering, J. Magn. Magn. Mater. 480 (2019) 171-185.

[13]V.A. Ferreira, D. Toscano, S.A. Leonel, P.Z. Coura, R.A. Dias, F. Sato, Transverse domain wall scattering and pinning by magnetic impurities in magnetic nanowires, J. Appl. Phys. 114 (2013) 013907.

[14]D. Toscano, S.A. Leonel, P.Z. Coura, F. Sato, B.V. Costa, M. Vázquez, Magnetization reversal of the transverse domain wall confined between two clusters of magnetic impurities in a ferromagnetic planar nanowire, J. Magn. Magn. Mater. 419 (2016) 37-42.

[15]C.I.L. de Araujo, J.C.S. Gomes, D. Toscano, E.L.M. Paixão, P.Z. Coura, F. Sato, D.V.P. Massote, S.A. Leonel, Investigation of domain wall pinning by square anti-notches and its application in three terminals MRAM, Appl. Phys. Lett. 114 (2019) 212403.
